# Supplementary material for: Taming geometric frustration by leveraging structural elasticity
Source: arXiv:2106.01535 ancillary file (2021-06-03)
Supplement: Supplementary file 1 [file SupplementaryMaterial.pdf]

## Supplementary Information

### Taming geometric frustration by leveraging structural elasticity

Janav P. Udani and Andres F. Arrieta\*

*Purdue University*

(Dated: June 3, 2021)

#### **This file includes:**

1. Materials and Methods
2. Definitions of the different length scales involved in the analysis of the dome patterned metasheets
3. Rayleigh-Ritz model for investigating the topology of an inverted axisymmetric unit
4. Comparison between the axisymmetric mirror-buckled inversion mode v/s elliptically post-buckled inversion mode
5. Experimental images of the hierarchically multistable states of the  $5 \times 5$  square metasheet
6. Geometric frustration and hierarchical multistability in a Nylon metasheet
7. List of Supplementary Videos

---

\* aarrieta@purdue.edu

## I. MATERIALS AND METHODS

### A. Experimental Specimen Design and Manufacturing

The experimental specimens are manufactured using Fused Deposition Modeling (FDM) 3D printing. The specimens are first modelled in SolidWorks 2016. The 3D files are then sliced using Ultimaker Cura 4.3.0 and printed on an Ultimaker 3+ using white thermoplastic polyurethane, supplied as Ultimaker TPU 95A (white). The specimens are printed flat on the print bed with material extruded from a single nozzle.

### B. Details on Finite Element (FE) Analyses

For the FE analysis, the specimens are modelled using Abaqus/CAE 2018 and Python scripting. A linear-elastic material formulation for TPU is employed for the simulations with an elastic modulus of 51MPa and Poisson's ratio 0.3. The effective elastic modulus for Ultimaker TPU 95A (white) is determined by conducting dogbone tests in-line with the ASTM D638 standard (Fig. S1). The simulation consists of multiple loading steps for dome inversion and each loading step is followed by two/three relaxation steps to allow the sheet to relax after each inversion event. Additionally, the metasheets are pinned at the centre over the entire simulation to avoid any rigid body motion. The specimens are then meshed with

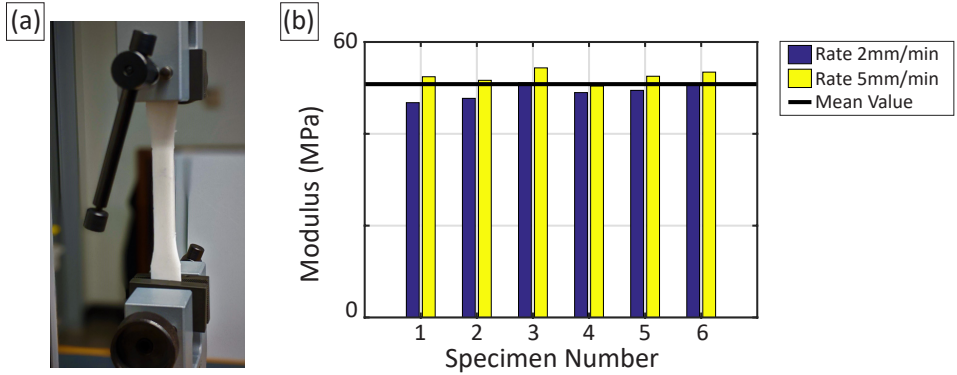

FIG. S1: (a) Dogbone test for determining the modulus of white Ultimaker TPU 95A. (b) Post-processed results indicating the modulus for 6 different specimens, each tested under two different loading rates.

a seed size of  $\leq 2\text{mm}$  using a quad-dominated mesh (shell elements). Diving into the loading details, individual domes are sequentially inverted in each loading step (Dome 1 in LoadStep-1, Dome2 in LoadStep-2, and so on) by an applied displacement (velocity)-load at the domes' centre while constraining the internal and external edges of the specimen. The boundary conditions are released in the subsequent relaxation steps to allow the specimen to relax in the deformed global configuration following each dome inversion cycle, thus simulating a programmed sequence of dome inversion events on the metasheet. Numerical damping factor values of  $\leq 10^{-6}$  are defined for each step in the simulation. Finally, the simulations are solved with Abaqus/Standard (implicit formulation) on the Brown community cluster at Purdue University. A single node on the Brown cluster features 24 processor cores and 96 GB of RAM.

For the higher-order frustrated states in Fig. 2 in the main manuscript, following dome inversion and subsequent relaxation, small loads are applied at specific control points on the metasheet. The location and orientation of these small displacement loads are chosen to favor one of the co-existing hierarchical states. The sheet is again allowed to relax after load application and is allowed to settle in the desired stable hierarchical state.

For the  $3 \times 3$  and  $5 \times 5$  metasheets' ground state configurations (Figs. 2, 4 and 5 in the main manuscript), the specimens exhibit self-contact when all the domes are inverted. To account for this, General contact (Standard) interaction property is defined for the respective metasheets. The self-contact formulation models frictionless tangential behavior and the system default normal contact behavior, i.e., "hard" contact pressure-overclosure and default constraint enforcement method. Additionally, to render the  $5 \times 5$  metasheet simulations time efficient, the solver formulation is switched to Dynamic-Implicit, Quasi-Static for all of the loading steps and some of the relaxation steps. Accordingly, we use a density of  $1.22 \text{ g/cm}^3$  for the material formulation [1].

### C. Details on Analytical Modelling

We use the symbolic manipulation software Wolfram Mathematica 9 for implementing both of the analytical formulations employed in this work, i.e., the homogenisation model for finding the dominant global deformation modes and the Rayleigh-Ritz model for investigating the topology of the deformed axisymmetric units. The models are solved for

in Mathematica and the data is subsequently exported for plotting and post-processing in MATLAB R2016b.

#### **D. Dimensions of specimens employed in the manuscript figures**

##### *1. $3 \times 3$ square metasheets*

The  $3 \times 3$  square metasheets illustrated in Figs. 2, 4 and 5 in the main manuscript feature dome units with dome base radius,  $R = 8$  mm, dome height,  $h = 5$  mm, unit thickness  $t = 0.7$  mm, and unit side length,  $SS = 22.4$  mm. For the square metasheets, the unit side length is equal to the spacing between two nearest neighbor dome centres.

##### *2. Unit cell buckling analysis*

The specimens employed for the unit cell buckling analysis in Fig. 3 in the main manuscript have dimensions,  $R = 8$  mm,  $h = 5$  mm and,  $t = 0.5$  mm. The three different planform area values for the flat regions are  $A_1 \approx 122.93 \text{ mm}^2$ ,  $A_2 \approx 282.93 \text{ mm}^2$  and,  $A_3 \approx 582.93 \text{ mm}^2$ .

##### *3. Hexagonal metasheets*

The hexagonal metasheets in Fig. 3 in the main manuscript have dimensions  $R = 8$  mm,  $h = 4$  mm,  $t = 0.5$  mm and spacing between two nearest neighbor dome centres,  $SS = 23.2$  mm.

##### *4. $5 \times 5$ square metasheets*

The  $5 \times 5$  square metasheets in Figs. 4 and 5 in the main manuscript have dimensions  $R = 8$  mm,  $h = 4$  mm,  $t = 0.5$  mm, and  $SS = 22.4$  mm.

### 5. *Random pattern metasheet*

The random pattern metasheet in Fig. 4 in the main manuscript has dimensions,  $R = 8$  mm,  $h = 4$  mm and,  $t = 0.4$  mm.

### 6. $8 \times 8$ *square metasheet*

The  $8 \times 8$  square metasheet in Fig. 4 in the main manuscript has dimensions  $R = 8$  mm,  $h = 5$  mm,  $t = 0.625$  mm and  $SS = 20.8$  mm.

### 7. *Specimens for studying hierarchical multistability boundaries*

The specimens in Figs. S3 and S5 have dimensions  $R = 8$  mm,  $h = 5$  mm,  $t = 0.625$  mm and  $SS$  is varied.

## II. DEFINITIONS OF THE DIFFERENT LENGTH SCALES INVOLVED IN THE ANALYSIS OF THE DOME PATTERNED METASHEETS

The dome patterned metasheets analyzed in this study are characterised by a hierarchical structure spanning three different length scales (Fig. S2). Characteristic features at each of the three length scale combine together to allow for the unique property-set and hierarchical multistable behavior at the global scale. Accordingly, the different length scales are defined as:

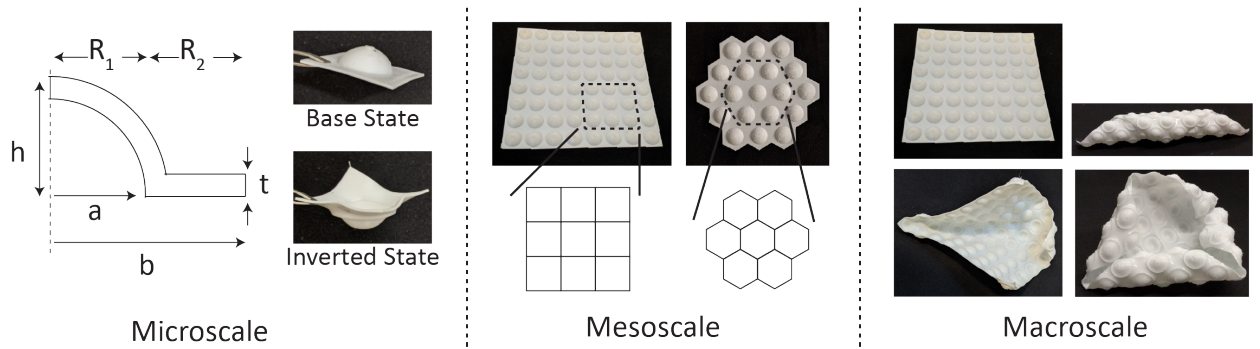

FIG. S2: The different length scales involved in the design and analyses of the hierarchical metasheets.

1. **Microscale** - The microscale comprises the individual units. The local dome dimensions and the dimensions of the flat region constitute the microscale design. Additionally, the inversion of the domes and the local post-buckling behavior of individual units are also microscale features.
2. **Mesoscale** - The mesoscale consists of the patterning of the local dome units. For example, the square and hexagonal patterned metasheets featuring identical dome units are distinguished from each other at the mesoscale. Similarly, regular v/s irregular tessellations, ordered v/s random patterns are all mesoscale design parameters.
3. **Macroscale** - The macroscale characterises the global behavior of the metasheet. The globally deformed configurations that the metasheet assumes as the domes are inverted constitute the macroscale. Accordingly, the hierarchical states are distinguished from each other at the macroscale.

### III. RAYLEIGH-RITZ MODEL FOR INVESTIGATING THE TOPOLOGY OF AN INVERTED AXISYMMETRIC UNIT

Geometric frustration in our metasytem and the ensuing hierarchical multistability characteristics only manifest when a sufficient degree of pre-stress is inputted into the system, as with the temperature-driven degenerate bending plates [2, 3]. This invariably corresponds to the pre-stress introduced via dome inversion and its propensity to introduce preferential bending directions in the dome metasheets. If the domes are packed in a sparse manner, the metasheet in the all domes inverted state assumes a non-developable, bent configuration, qualitatively similar to that seen for low thermal field values in the bending plates (Fig. S3a). As the packing density of the domes is increased beyond a certain threshold, the metasheet bifurcates into a developable form as the domes are inverted in the system. We identify the packing ratio, i.e., the ratio of the unit side length ( $S$ ) to the radius of the dome ( $R$ ), ( $PK = \frac{S}{R}$ ) as a critical parameter governing this bifurcation in the metasheets. This observation stems from the fact that inversion of a dome results in axisymmetric out-of-plane bending of the flat region surrounding the dome. This axisymmetric out-of-plane deformation field interacts with the non-axisymmetrically shaped boundary leading to the non-uniform bending resistance central to the manifestation of the preferential bending di-

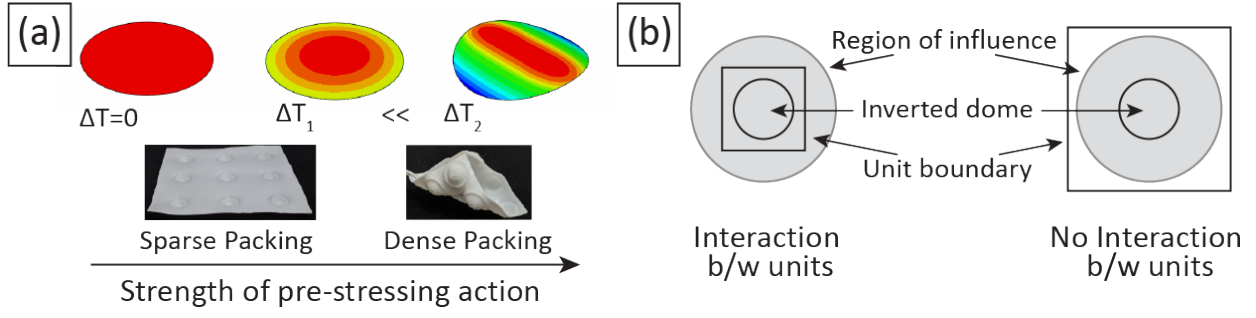

FIG. S3: (a)-(b) Geometric frustration manifests only when the domes are sufficiently densely packed and the region of influence of the deformation field following dome inversion exceeds beyond the unit boundary.

reactions at the macroscale. However, if the packing factor is sufficiently large, such that the flat region of any given unit extends beyond the radius of influence of the inversion-induced field, the interplay between the non-axisymmetric boundary shape and the axisymmetric deformation field is lost (Fig. S3b). This excess region offers largely uniform bending resistance in all directions and, consequently, the metasheet loses preferential bending directions and starts behaving like a flat sheet subjected to external loading.

We capture this bifurcation between hierarchical to non-hierarchical global behavior employing an analytical approach modelling the topology of an axisymmetric unit in the inverted state. Specifically, we model the topology as the microscale packing factor  $PK$  is varied, inspecting the change in the gradient ( $\lambda_r$ ) at the flat region's boundary for each design. A zero-crossing in the  $\lambda_r(PK)$  plot marks the limit beyond which the flat region topology is unaffected by the inversion induced deformation field, thereby indicating the loss of hierarchical multistability.

We employ the Föppl-von Kármán equations (assuming axisymmetry) in the radial co-ordinates  $r$  and  $\theta$ ,

$$D\nabla^4 w - \frac{t}{r} \frac{\partial}{\partial r} \left[ \frac{\partial w}{\partial r} \frac{\partial \Phi}{\partial r} \right] = 0 \quad \& \quad \frac{\nabla^4 \Phi}{E} + \frac{1}{r} \frac{\partial w}{\partial r} \frac{\partial^2 w}{\partial r^2} = 0, \quad (1)$$

where,  $D = \frac{Et^3}{12(1-\nu^2)}$  is the flexural rigidity, and  $\Phi$  and  $E$  are the Airy's stress function and elastic Young's modulus respectively. Following Ref. [4], we decouple equations (1) into their stretching and bending components and solve for the stable states by Rayleigh-Ritz minimisation of the total potential energy.

The unit is divided into two distinct regions - (i) the central initially curved dome; and

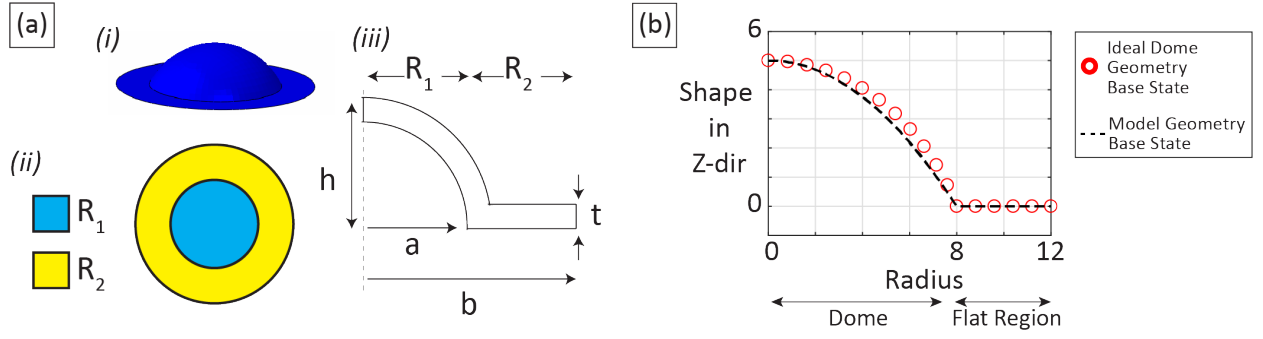

FIG. S4: (a) (i) The axisymmetric dome unit. (ii)-(iii) The different design parameters and the regions  $R_1$  and  $R_2$  involved in the analysis. (b) Topology of the axisymmetric unit employed in the analytical model as compared to the ideal dome geometry. The red markers correspond to the actual dome geometry. The black dashed line corresponds to the mathematical function approximating the dome geometry that is employed for the analytical model.

(ii) the surrounding flat region (Fig. S4a). We start by assuming an initially curved shape for the unit as,

$$w_{R1}^0 = (1 - \rho^2)w_m^0 \quad \& \quad w_{R2}^0 = 0, \quad (2)$$

where,  $w_{R1}^0$  and  $w_{R2}^0$  are the initial displacements of the central dome and the flat region respectively,  $\rho = \frac{r}{a}$  is the dimensionless radial parameter, with  $a$  being the base diameter of the dome and  $w_m^0$  is the initial midpoint deflection of the dome. The geometry assumed in equation (2) is an approximation of the ideal dome geometry. Nonetheless, the results are found to be in good agreement with the actual dome FE results (see Fig. S4b and Fig. S5). As discussed in the main manuscript, the initial or the base state of the unit is stress-free. Next, we denote the displacement of the inverted, stressed configuration by  $w_{R1}$  and  $w_{R2}$  for the dome and the flat region respectively. Accordingly, the change in displacement is given by  $\hat{w}_{R1} = w_{R1} - w_{R1}^0$  and  $\hat{w}_{R2} = w_{R2} - w_{R2}^0$  respectively. The gradient ( $\lambda_r$ ), radial and circumferential curvature ( $\kappa_r$  and  $\kappa_\theta$ ) terms are derived from the displacement expressions for the respective states as,

$$\lambda_r = -\frac{dw}{dr} \quad , \quad \kappa_r = -\frac{d^2w}{dr^2} \quad \& \quad \kappa_\theta = -\frac{1}{r} \frac{dw}{dr}, \quad (3)$$

and the variations in the respective terms ( $\hat{\lambda}_r$ ,  $\hat{\kappa}_r$  and  $\hat{\kappa}_\theta$ ) between the initial and the final states follow naturally. Correspondingly, the principal bending moments and the shear stress

terms are defined as,

$$m_r = D(\kappa_r + \nu\kappa_\theta) \quad , \quad m_\theta = D(\kappa_\theta + \nu\kappa_r) \quad \& \quad q_r = \frac{dm_r}{dr} + \frac{m_r - m_\theta}{r}, \quad (4)$$

where,  $\nu$  is the Poisson's ratio and linear elastic, isotropic material behavior is assumed. Again, since the base state is stress free, the change in the respective quantities in equation (4) is equal to the final value of the quantities, i.e.,  $\hat{m}_r = m_r$ ,  $\hat{m}_\theta = m_\theta$  and  $\hat{q}_r = q_r$ . Lastly, all of the quantities in equations (3) and (4) are calculated for both of the dome and the flat regions, i.e.,  $R1$  and  $R2$ .

For the Rayleigh-Ritz formulation, we assume a polynomial series expansion for the change in the radial curvature for both of the regions in the unit, i.e.,  $\hat{\kappa}_r = \sum_{i=0}^n c_i r^i$ , and the other quantities are then calculated in terms of the generalised co-ordinates,  $c_i$ . This results in two additional constants for each region in their respective displacement expressions originating due to the double integration operation for transforming between the two fields. These additional constants are satisfied by imposing the boundary conditions (BC) and continuity conditions in the out-of-plane problem. For this formulation, we assume that the unit is pinned at its outermost boundary. This assumption is an idealisation of the more realistic spring-type BC that is levied by the surrounding elastic continuum on any given unit in the metasheet. However, we find that the results obtained by following a pinned outer edge BC allow for a conservative estimate of the limits on hierarchical multistability in our metasheets. A more precise bound can be obtained by augmenting the model in it's current form with springs assumed at the edges. The pinned BC for the out-of-plane problem can be mathematically expressed as,

$$w_{R2}|_{r=b} = 0 \quad \& \quad m_{r-R2}|_{r=b} = 0. \quad (5)$$

Additionally, for the full dome with no slits/cuts, we have two other conditions for the centre point of the unit that are expressed as,

$$q_{r-R1}|_{r=0} = 0 \quad \& \quad \left. \frac{\partial w_{R1}}{\partial r} \right|_{r=0} = 0. \quad (6)$$

These BCs for the out-of-plane problem (equations (5) and (6)) are further augmented by considering the elastic continuity conditions for the displacement and the slope at the boundary connecting the dome to the surrounding flat region,

$$w_{R1}|_{r=a} = w_{R2}|_{r=a} \quad \& \quad \left. \frac{\partial w_{R1}}{\partial r} \right|_{r=a} = \left. \frac{\partial w_{R2}}{\partial r} \right|_{r=a}. \quad (7)$$

This set of six constraint equations in the out-of-plane problem is first employed to solve for the four constants resulting from the double integration operation to find the displacement fields from the assumed curvature expressions. The remaining constraint expressions are satisfied by reducing the number of degrees of freedom by the corresponding amount. For example, for the full dome shell, considering only even terms in the assumed curvature expression automatically satisfies the BC for the shear force (equation (6)), thus simplifying the model and improving the computational efficiency. Additionally, we find that considering four terms in the assumed curvature fields for each of the regions allows for sufficient accuracy in modelling the topology of the inverted unit. Accordingly, the assumed expressions for the change in the radial curvature are given as,

$$(\hat{\kappa}_r)_{R1} = \sum_{i=0}^4 (c_i)_{R1} r_{R1}^{2i} \quad \& \quad (\hat{\kappa}_r)_{R2} = \sum_{i=0}^4 (c_i)_{R2} r_{R2}^i. \quad (8)$$

Next, moving on to the in-plane problem, we employ the Airy's stress function,  $\Phi$ , for describing the mid-plane stress resultants ( $\sigma_r$  and  $\sigma_\theta$ ) as

$$\sigma_r = \frac{1}{r} \frac{d\Phi}{dr} \quad \& \quad \sigma_\theta = \frac{d^2\Phi}{dr^2}. \quad (9)$$

The corresponding in-plane strains ( $\epsilon_r$  and  $\epsilon_\theta$ ) are given as,

$$\epsilon_r = \frac{1}{E}(\sigma_r - \nu\sigma_\theta) \quad \& \quad \epsilon_\theta = \frac{1}{E}(\sigma_\theta - \nu\sigma_r). \quad (10)$$

The nonlinearity associated with the dome inversion and the ensuing bistable behavior is modelled by using nonlinear strain-displacement relationships that allow for large displacements but maintain low strains. This relationship is expressed in the radial co-ordinates as

$$\epsilon_r = \frac{du_r}{dr} + \left[ \frac{1}{2} \left( \frac{dw}{dr} \right)^2 - \frac{1}{2} \left( \frac{dw^0}{dr} \right)^2 \right] \quad \& \quad \epsilon_\theta = \frac{u_r}{r}. \quad (11)$$

In order to express the in-plane stresses and strains purely in terms of the generalised co-ordinates, we model the stretching-bending interaction by connecting the change in Gaussian curvature to the in-plane strains and by extension, the Airy's stress function as

$$-E\hat{g} = \frac{d^4\Phi}{dr^4} + \frac{2}{r} \frac{d^3\Phi}{dr^3} - \frac{1}{r^2} \frac{d^2\Phi}{dr^2} + \frac{1}{r^3} \frac{d\Phi}{dr}. \quad (12)$$

Solving this equation, the complete solution for each region consists of the homogeneous solution (expressed in terms of  $r$ ) and the particular solution, that is expressed as,

$$D_1 + D_2 \text{Log}[r] + \frac{1}{2} D_3 r^2 + D_4 r^2 \left( -\frac{1}{4} + \frac{1}{2} \text{Log}[r] \right). \quad (13)$$

We note that four additional constants are added in the respective solutions for each region. Taking derivatives to find the mid-plane stress resultants, these constants subsequently appear in the respective expressions in the following form,

$$\sigma_r = D_2 \frac{1}{r^2} + D_3 + D_4 \text{Log}[r] + \dots \quad \& \quad \sigma_\theta = -D_2 \frac{1}{r^2} + D_3 + D_4 (1 + \text{Log}[r]) + \dots \quad (14)$$

This set of six additional constants (three for each region) is solved for by employing the in-plane boundary conditions and the in-plane continuity conditions. To begin with, the stress at the centre of the dome ( $R1$ ) cannot be infinite. Hence,  $(D_2)_{R1} = (D_4)_{R1} = 0$ . Next, using the expressions for  $\epsilon_r$  and  $\epsilon_\theta$ , we obtain two distinct expressions for the in-plane displacement field,  $u_r$  for the flat region,  $R2$ . However, for real solutions to the problem, both of the obtained expressions for the displacement fields need to be compatible with each other. Solving for the ensuing compatibility equation,  $[u_r(\epsilon_r)]_{R2} = [u_r(\epsilon_\theta)]_{R2}$ , the constant  $(D_4)_{R2}$  is determined. The remaining three constants  $(D_3)_{R1}$ ,  $(D_2)_{R2}$  and  $(D_3)_{R2}$  are determined by solving for the in-plane pinned BC at the outer edge,

$$(u_r)_{R2} \Big|_{r=b} = 0, \quad (15)$$

and the continuity conditions for the in-plane displacement and the circumferential stress at the shared boundary,

$$(u_r)_{R1} \Big|_{r=a} = (u_r)_{R2} \Big|_{r=a} \quad \& \quad (\sigma_\theta)_{R1} \Big|_{r=a} = (\sigma_\theta)_{R2} \Big|_{r=a}. \quad (16)$$

With these simplifications, all of the quantities in the in-plane and out-of-plane problem are unambiguously expressed purely in terms of the generalised co-ordinates,  $c_i$ , and the radial co-ordinate,  $r$ . The bending and stretching energy contributions ( $\Pi_B$  and  $\Pi_S$ ) for each of the two regions can be subsequently expressed as,

$$\Pi_B = \frac{1}{2} \int_{\Omega} (\hat{\kappa}_r m_r + \hat{\kappa}_\theta m_\theta) dA \quad \& \quad \Pi_S = \frac{t}{2} \int_{\Omega} (\epsilon_r \sigma_r + \epsilon_\theta \sigma_\theta) dA. \quad (17)$$

Adding the bending and stretching energy contributions for both the dome and the flat region ( $\Pi = (\Pi_B)_{R1} + (\Pi_S)_{R1} + (\Pi_B)_{R2} + (\Pi_S)_{R2}$ ), local minima in the total potential energy expression are determined by employing the *FindMinimum* function in Mathematica. These local minimum energy points correspond to equilibrium configurations of the unit, i.e., the base state and the inverted state. The stability of each of the equilibrium points is confirmed by evaluating the positive definiteness of the Hessian Matrix  $H_{ij} = \frac{\partial^2 \Pi}{\partial c_i \partial c_j}$ .

For generality and in order to improve the computational efficiency of the model, we express the unit geometry in terms of three non-dimensional parameters - the shallowness ( $SH = h/a$ ), slenderness ( $SL = h/t$ ) and packing factor ( $PK = 2b/a$ ). Additionally, we non-dimensionalise the field variables for both the regions  $R1$  and  $R2$  in the following manner,

$$\rho = \frac{r}{a} \quad , \quad \omega = \frac{w}{t} \quad , \quad K = \kappa \frac{a^2}{t} \quad , \quad S = \frac{\sigma a^2}{Et^2} \quad \& \quad M = \frac{ma^2}{Et^4}. \quad (18)$$

Lastly, the generalised co-ordinates,  $c_i$  are also normalised by the dome base radius  $a$  to further improve the computational efficiency of the model. The normalised set of generalised co-ordinates is defined as

$$\hat{c}_i = \frac{c_i}{a}. \quad (19)$$

The results for the unit topology and for predicting the limit of hierarchical multistability in our metasheets are illustrated in Fig. S5, and are found to be in good agreement with experimental results.

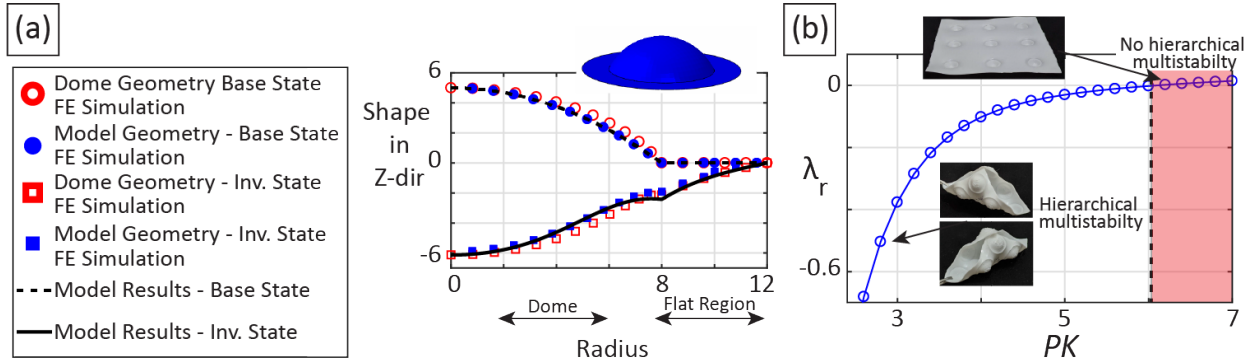

FIG. S5: (a) Topology of the inverted axisymmetric unit as predicted by the analytical model and FE simulations. The red markers correspond to FE results for the actual dome geometry. The blue markers correspond to FE results for the mathematical function approximating the dome geometry that is employed for the analytical model (equation (2)). (b)  $\lambda_r(PK)$  plot illustrating the model predicted boundary separating hierarchical and non-hierarchical design regimes. The insets illustrate experimental examples of the respective designs.

#### IV. COMPARISON BETWEEN THE AXISYMMETRIC MIRROR-BUCKLED INVERSION MODE V/S ELLIPTICALLY POST-BUCKLED INVERSION MODE

The static bistability of doubly-curved shells or domes has been extensively studied and analyzed in literature [4–11]. The dominant deformation mode involved in dome inversion is the axisymmetric mirror-buckled mode. However, while the second stable state is largely axisymmetric, asymmetric configurations have been found to emerge while the dome is transitioning from one state to the other [10, 12]. These asymmetric modes have been largely studied under the context of the dome deformation when subjected to a point load at the apex. Notably, higher order polygonal post-buckling modes have been found during such localised loading cases [10, 12, 13]. These higher order polygonal modes feature a

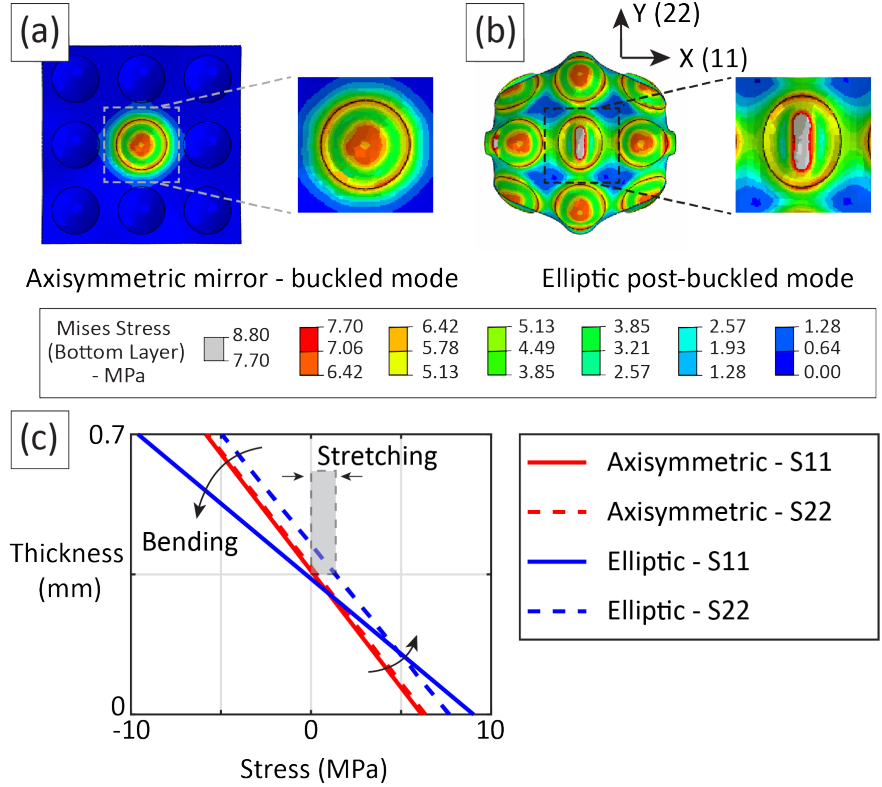

FIG. S6: (a) The axisymmetric mirror-buckled deformation mode when a single dome is inverted in the metasheet. (b) The elliptic post-buckled deformation mode on the centre dome when all domes are inverted and the metasheet assumes a higher order frustrated state. (c) The through-thickness stress fields for the centre point on the centre dome for the metasheet deformation states in (a) and (b).

strong stretching-bending interaction as compared to the mirror-buckled mode, where the deformation is largely bending-dominated [9, 10, 13]. As illustrated in Figs 2, 3 in the main manuscript, we find these higher order post-buckling modes in our system as well, although these appear in a qualitatively different context. In our system, such modes emerge due to the asymmetry in the design of the unit planform geometry and are found to originate from the unit boundary. Consequently, they start to localise away from the dome centre as the mesoscale packing factor is increased. Importantly, these higher order post-buckled modes play a crucial role in the hierarchical multistable behavior in our metasheets. A single dome inverted in any metasheet features a largely axisymmetric shape and assumes the mirror-buckled configuration (Fig. S6a). However, we notice that as an increasing number of domes are inverted in the metasheet, interactions start developing between neighboring inverted units. This results in post-buckled shapes that are driven by - (i) the unit geometry; (ii) the state of the neighboring units; and (iii) the sequence in which the interactions are imposed. This feature is distinctly seen on the centre dome in the higher-order frustrated state for a  $3 \times 3$  metasheet, as illustrated in Fig. S6b. The centre dome's deformation state departs from the axisymmetric mirror-buckled state and assumes an elliptical post-buckled shape with major axis aligned with the vertical (Y-direction) dimension of the metasheet. Analyzing the through-thickness stress fields in the X- (11) and Y-directions (22) for the centre point of the respective units (Fig. S6c), we find that for the axisymmetric mode, the through-thickness fields are qualitatively similar and are bending dominated. In contrast, for the higher-order frustrated state, the axisymmetry is clearly lost with the stress-fields in the respective directions exhibiting qualitatively different behavior. Furthermore, the stretching-bending interaction for the elliptic post-buckled shape is apparent for the through-thickness field in the Y-direction, in contrast to the mirror-buckled state where this feature is absent and the deformation is bending dominated. This distinct switching behavior between purely bending dominated to a combined stretching-bending deformation state controls the symmetry breaking of the post-buckled mode on the individual domes. These interactions between the stretching and bending behavior within the microstructure of our metasheets are central for the manifestation of macroscale geometric frustration and hierarchical multistable behavior.

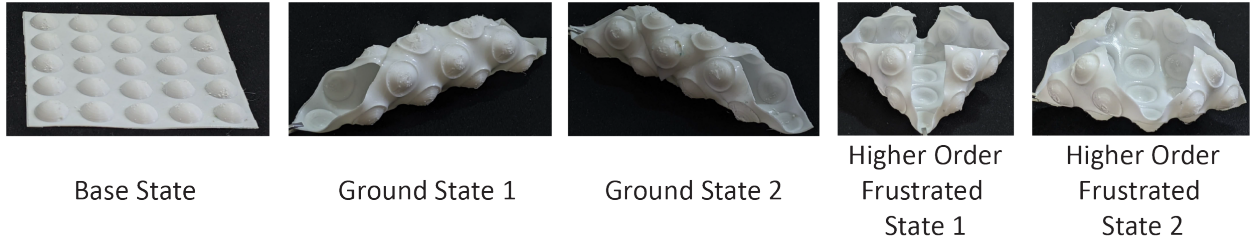

FIG. S7: Experimental images of the base state and the hierarchical multistable states when all domes are inverted for the  $5 \times 5$  square metasheet.

## V. EXPERIMENTAL IMAGES OF THE HIERARCHICALLY MULTISTABLE STATES OF THE $5 \times 5$ SQUARE METASHEET

The base state and four hierarchical multistable states for the  $5 \times 5$  metasheet when all domes are inverted are illustrated in Fig. S7 .

## VI. GEOMETRIC FRUSTRATION AND HIERARCHICAL MULTISTABILITY IN A NYLON METASHEET

The manifestation of macroscale geometric frustration, and the ensuing hierarchically multistable behavior of our metasheets are purely geometric features and independent of the material properties as long as the dome inversion-induced stresses are within the failure limits for the corresponding material. We demonstrate this by employing a Nylon metasheet consisting of domes arranged in a  $3 \times 3$  square pattern (Fig. S8a). Nylon has an elastic modulus of 579 MPa, i.e. is  $22\times$  more than TPU [14]. With a glass transition temperature above  $50^\circ$  C, Nylon shows no viscoelastic effect at room temperature. All domes in the Nylon-made metamaterial sheet have uniform dimensions with height  $h = 4$  mm, base radius  $R = 12$  mm, thickness  $t = 0.4$  mm and unit side length  $SS = 28$  mm. Locally, each individual dome features two stable configurations: the as-printed base state and the inverted state. At the global scale, the nylon sheet is again found to exhibit hierarchical multistability with the emergence of the ground states (Fig. S8b) and the higher-order frustrated states (Fig. S8c) when all the domes are inverted. This result indicates that geometric frustration and the ensuing hierarchical multistability features are manifested purely due to the geometry of the metasheets and are compatible with different material

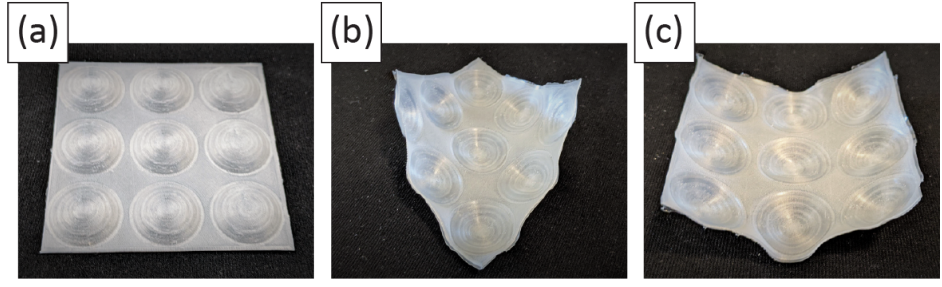

FIG. S8: Experimental images of the base state and the hierarchical multistable states when all domes are inverted for the  $3 \times 3$  Nylon metasheet.

chemistries. Concretely, material viscoelastic effects observed in many of the soft material systems are not necessary for hierarchical multistability to emerge.

## VII. LIST OF SUPPLEMENTARY VIDEOS

1. Inversion of a single dome unit.
2. Shifting between the hierarchically multistable states of a  $3 \times 3$  square metasheet by means of external loads.
3. The hierarchically multistable states of a hexagonal patterned metasheet
4. Diagonal dome inversion sequence leading to a ground state on a  $3 \times 3$  square metasheet.
5. Symmetric dome inversion sequence leading to a higher order frustrated state on a  $3 \times 3$  square metasheet.
6. Inversion sequence leading to a higher order frustrated state on a  $5 \times 5$  square metasheet.

---

[1] Ultimaker, Technical data sheet - Ultimaker TPU 95A, , 1 (2018).

[2] E. H. Mansfield, Bending, buckling and curling of a heated thin plate, Proceedings of the Royal Society of London. Series A. Mathematical and Physical Sciences **268**, 316 (1962).

- [3] E. H. Mansfield, Bending, buckling and curling of a heated elliptical plate, Proceedings of the Royal Society of London. Series A. Mathematical and Physical Sciences **288.1414**, 396 (1965).
- [4] P. M. Sobota and K. A. Seffen, Effects of boundary conditions on bistable behaviour in axisymmetrical shallow shells, Proceedings of The Royal Society A **473**, 20170230 (2017).
- [5] E. L. Reiss, H. J. Greenberg, and H. B. Keller, Nonlinear Deflections of Shallow Spherical Shells, Journal of the Aeronautical Sciences **24**, 533 (1957).
- [6] H. B. Keller and E. L. Reiss, Spherical Cap Snapping, Journal of the Aerospace Sciences **26**, 643 (1959).
- [7] G. W. Brodland and H. Cohen, Deflection and snapping of spherical caps, International Journal of Solids and Structures **23**, 1341 (1987).
- [8] A. Brinkmeyer, M. Santer, A. Pirrera, and P. M. Weaver, Pseudo-bistable self-actuated domes for morphing applications, International Journal of Solids and Structures **49**, 1077 (2012).
- [9] K. A. Seffen and S. Vidoli, Eversion of bistable shells under magnetic actuation : a model of nonlinear shapes, Smart Materials and Structures **25**, 065010 (2016).
- [10] M. Taffetani, X. Jiang, D. P. Holmes, and D. Vella, Static bistability of spherical caps, Proceedings A (2018).
- [11] L. Stein-Montalvo, P. Costa, M. Pezzulla, and D. P. Holmes, Buckling of geometrically confined shells, Soft Matter **15**, 1215 (2019).
- [12] J. R. Fitch, The buckling and post-buckling behavior of spherical caps under concentrated load, International Journal of Solids and Structures **4**, 421 (1968).
- [13] A. Vaziri and L. Mahadevan, Localized and extended deformations of elastic shells, Proceedings of the National Academy of Sciences **105**, 7913 (2008).
- [14] Ultimaker, Technical data sheet: Nylon, , 1 (2017).
